# Supplementary material for: Local control and lateral nanofocusing of hyperbolic phonon polaritons
Source: arXiv:2604.08996 source file (2026-04-10)
Supplement: Supplementary file 1 [file si_setup.tex]

%-----PACKAGES-----
\usepackage{orcidlink}
\usepackage{hyperref}
\hypersetup{colorlinks,
	linkcolor={blue!75!black!80!yellow},
	citecolor={blue!75!black!80!yellow},
	urlcolor={blue!75!black!80!yellow},
	pdfstartview=FitH}
\usepackage[top=35mm, bottom=35mm, left=35mm, right=35mm]{geometry} % change margins
\usepackage{graphicx}
\usepackage{tabularx}
\usepackage{mathrsfs}
\usepackage{xspace}
\usepackage{braket}
\usepackage{xr}
\usepackage{xcite}
\usepackage{xcolor,soul}
\usepackage{stmaryrd} % provides \llbracket and \rrbracket for difference-operations
\usepackage[UKenglish]{babel}
\usepackage{enumitem} % allows changing enumerate bullets
\usepackage{diagbox}
\usepackage{float}
\usepackage{physics}
\usepackage{empheq} % for numbering different cases in an equation
\usepackage{bbm}

\usepackage{siunitx}
\sisetup{range-phrase =\text{\,--\,},
		 list-units   =single,
	 	 range-units  =single,
		 list-pair-separator = {\ \text{and}\ },
		 list-separator = {,\ \linebreak[0]},
		 list-final-separator = {,\ \linebreak[0]\text{and}\ },
	 	 detect-all = true}
\DeclareSIUnit[number-unit-product=]\percent{\char`\%} % remove space before percentage "units"

%-----APPPEND 'S' TO REFERENCES OF ALL KINDS-----
 % equations
\renewcommand{\thetable}{S\arabic{table}} % tables
\renewcommand{\thefigure}{S\arabic{figure}} % figures
 % citations

 % change appearance of description lists

%-----LOADING RELEVANT FONTS [Times Roman]-----
\usepackage{txfonts}  % Times Roman fonts
\usepackage{txfontsb} % addition for txfonts, including old style numerals and greek

%-----REDEFINE THE RMP STYLE OF AUTHORS AND AFFILIATIONS-----
\makeatletter
\def\frontmatter@authorformat{%
	\preprintsty@sw{\vskip0.5pc\relax}{}%
	\@tempskipa\@flushglue
	\@flushglue\z@ plus50\p@\relax
	\raggedright\advance\leftskip.25in\relax
	\@flushglue\@tempskipa
	\parskip\z@skip
}%
\def\frontmatter@affiliationfont{% Helvetica 9/10.2
	\small\slshape\selectfont\baselineskip10.5\p@\relax
	\@tempskipa\@flushglue
	\@flushglue\z@ plus50\p@\relax
	\raggedright\advance\leftskip.25in\relax
	\@flushglue\@tempskipa
}
\def\paragraph{%
	\@startsection
	{paragraph}%
	{4}%
	{\parindent}%
	{\z@}%
	{-1em}%
	{\normalfont\small\itshape\textsf} % change so that paragraphs are also in sans serif font
}%
\renewcommand*\email[1][]{\begingroup\sanitize@url\@email{#1}} % remove the 'Electronic adress: ' from RMP style
\makeatother

\setcitestyle{numbers,square,sort&compress} % standard style square bracket, numbers style instead

% set figure and table caption title to bold... 
\makeatletter
\renewcommand*{\fnum@figure}{{\normalfont\bfseries \figurename~\thefigure}.}
\makeatother

\makeatletter
\renewcommand*{\fnum@table}{{\normalfont\bfseries \tablename~\thetable}.}
\makeatother

%----- Spacing and binary relations/operations -----
\thickmuskip=5mu plus 2mu minus 1mu  % binary relations (default, 5mu plus 5mu)
\medmuskip=4mu plus 2mu minus 2mu    % binary operations (default, 4mu plus 2mu minus 4mu)
\frenchspacing % ensure that revTeX does not do "double spaces" after punctuation

%-----Changing appearance of ToC-----
 % removing the automatic ToC name and removing line
\makeatletter
    \DeclareRobustCommand*{\deactivateaddvspace}{\let\addvspace\@gobble} % "deactivates" \addvspace command
    \DeclareRobustCommand*{\deactivatetocsubsections}{
    \def\l@subsection##1##2{}    % these definitions are inherited from \l@@sections, see 
    \def\l@subsubsection##1##2{} % ltxutils.dtx; "reset" them to remove subsections in ToC
    }
\makeatother

%----- Commands -----

% hack to fix revtex's toc (https://tex.stackexchange.com/a/631474/113831)
\makeatletter
\def\@sect@ltx#1#2#3#4#5#6[#7]#8{%
    \@ifnum{#2>\c@secnumdepth}{%
        \def\H@svsec{\phantomsection}%
        \let\@svsec\@empty
    }{%
        \H@refstepcounter{#1}%
        \def\H@svsec{%
            \phantomsection
        }%
        \protected@edef\@svsec{{#1}}%
        \@ifundefined{@#1cntformat}{%
            \prepdef\@svsec\@seccntformat
        }{%
            \expandafter\prepdef
            \expandafter\@svsec
            \csname @#1cntformat\endcsname
        }%
    }%
    \@tempskipa #5\relax
    \@ifdim{\@tempskipa>\z@}{%
        \begingroup
        \interlinepenalty \@M
        #6{%
            \@ifundefined{@hangfrom@#1}{\@hang@from}{\csname @hangfrom@#1\endcsname}%
            {\hskip#3\relax\H@svsec}{\@svsec}{#8}%
        }%
        \@@par
        \endgroup
        \@ifundefined{#1mark}{\@gobble}{\csname #1mark\endcsname}{#7}%
        \addcontentsline{toc}{#1}{%
            \@ifnum{#2>\c@secnumdepth}{%
                \protect\numberline{}%
            }{%
                \protect\numberline{\csname the#1\endcsname}%
            }%
            #7}% <<<<<<<<<<<<<<<<<<<<<<<< changed from #8
    }{%
        \def\@svsechd{%
            #6{%
                \@ifundefined{@runin@to@#1}{\@runin@to}{\csname @runin@to@#1\endcsname}%
                {\hskip#3\relax\H@svsec}{\@svsec}{#8}%
            }%
            \@ifundefined{#1mark}{\@gobble}{\csname #1mark\endcsname}{#7}%
            \addcontentsline{toc}{#1}{%
                \@ifnum{#2>\c@secnumdepth}{%
                    \protect\numberline{}%
                }{%
                    \protect\numberline{\csname the#1\endcsname}%
                }%
                #8}%
        }%
    }%
    \@xsect{#5}}%
\makeatother

% Section numbering
